# Supplementary material for: Know Thyself: Transferable Visual Control Policies Through Robot-Awareness
Source: arXiv:2107.09047 source file (2022-10-17)
Supplement: Supplementary file 2 [file supp_control_results.tex]

\begin{table}[h]
\caption{Tabletop pushing success rates for models pre-trained on multiple robots and transferred to the unseen Franka.}
\centering

\begin{tabular}{llc}
\toprule
Model & Cost & \thead{Zero-shot \\Franka }\\
\midrule
VFS & Pixel     &  6/18 (33\%)\\
RA & Pixel     & 0/18 (0\%) \\
VFS & RA     & 9/18 (50\%)\\
RA & RA   & \textbf{16/18} \textbf{(89}\%\textbf{)} \\
\bottomrule
\end{tabular}
\label{tab:supp_control_eval}
% \vspace{-4mm}
\end{table}
