# Supplementary material for: Know Thyself: Transferable Visual Control Policies Through Robot-Awareness
Source: arXiv:2107.09047 source file (2022-10-17)
Supplement: Supplementary file 3 [file supp_multiview_cost.tex]

\begin{table}
\caption{Simulated object pushing using either single-view or multi-view versions of the robot-aware cost.}
\centering
\begin{tabular}{llc}
\toprule
Cost & Success\\
\midrule
RA      & 95/100 (95\%) \\
RA (2 views)    & \textbf{98/100} (98\%) \\
\bottomrule
\end{tabular}

\label{tab:multiview_cost}
\end{table}
