# Supplementary material for: Know Thyself: Transferable Visual Control Policies Through Robot-Awareness
Source: arXiv:2107.09047 source file (2022-10-17)
Supplement: Supplementary file 5 [file supp_prediction_results.tex]

\begin{table}[h]
\caption{World dynamics model evaluations, reported as PSNR and SSIM over world regions.}
\centering
\begin{tabular}{@{}lcccc@{}}
\toprule
          Model & \multicolumn{2}{c}{\thead{Zero-shot \\ Mod. WidowX200}}  & \multicolumn{2}{c}{\thead{Zero-shot \\ Franka}} \\
\cmidrule(lr){2-3}
\cmidrule(lr){4-5}
&
\multicolumn{1}{c}{\thead{PSNR $\uparrow$}} &
\multicolumn{1}{c}{\thead{SSIM $\uparrow$}} &
\multicolumn{1}{c}{\thead{PSNR $\uparrow$}} &
\multicolumn{1}{c}{\thead{SSIM $\uparrow$}}   \\
\midrule
VF   &  31.40  & 0.924  & 28.31 & 0.901  \\
VFS   &  31.43 & 0.924 & 29.19 & 0.901  \\
RA-PL   &  31.54 & 0.923 & 28.84 & 0.895   \\
RA-L  & 31.67 & 0.923 & 29.13 & 0.903   \\
RA (Ours) & \textbf{32.12} & \textbf{0.929} & \textbf{29.37}  & \textbf{0.904}  \\
\bottomrule
\end{tabular}
\label{tab:supp_pred_eval}
\end{table}
